# Supplementary material for: Overcoming Multi-Model Forgetting
Source: arXiv:1902.08232 source file (2019-03-02)
Supplement: Supplementary file 1 [file appendix.tex]

% !TEX root = top_appd.tex
% !TEX spellcheck = en-US
\appendix

\section{Proofs}

%\MS{Try to find a way such that the lemma numbering starts from 1 again, so as to match the numbers in the main text. Also, please, copy the statements of the lemmas from the main text.}

%\MS{In appendix, I suggest we also explain how you get from Lemma 1 and Lemma 2 to Eq. 2.}

\begin{restatable}{lemma}{lemmaone}
	\label{lem1}
	Given a dataset $\mathcal{D}$ and two architectures with shared parameters $\vtheta_s$ and private parameters $\vtheta_1$ and $\vtheta_2$, and provided that $p(\vtheta_1, \vtheta_2 \mid \vtheta_s, \mathcal{D}) = p(\vtheta_1 \mid \vtheta_s, \mathcal{D})p(\vtheta_2 \mid \vtheta_s, \mathcal{D})$, we have
	\begin{equation}
	\label{eq:bayes2}
	p(\vtheta_1, \vtheta_2, \vtheta_s \mid \mathcal{D}) \propto \frac{p(\mathcal{D} \mid \vtheta_2, \vtheta_s) p(\vtheta_1, \vtheta_s) p(\vtheta_2, \vtheta_s)}{\int p(\mathcal{D} \mid \vtheta_1, \vtheta_s) p(\vtheta_1, \vtheta_s) d\vtheta_1}.\vspace{-2mm}
	\end{equation}
\end{restatable}

% \begin{lemma}
% Given a dataset $\gD$ and two architectures with shared \yb{parameters} $\theta_s$ and private ones $\theta_1$ and $\theta_2$, respectively, and under the assumption that $p(\theta_1, \theta_2 \mid \theta_s, \gD) = p(\theta_1 \mid \theta_s, \gD)p(\theta_2 \mid \theta_s, \gD)$, the posterior $p(\theta \mid \gD)$, with $\theta = (\theta_1, \theta_2, \theta_s)$, can be expressed as
% \begin{equation}
% \label{eq:bayes2}
% p(\theta \mid \gD) \propto \frac{p(\gD \mid \theta_2, \theta_s) p(\theta_1, \theta_s) p(\theta_2, \theta_s)}{\int p(\gD \mid \theta_1, \theta_s) p(\theta_1, \theta_s) d\theta_1}.
% \end{equation}
% \end{lemma}

\begin{proof}
Using Bayes' theorem and ignoring constants, we have %\footnote{The parameters are bold in the lemma but not the proof.  Is bold needed? actually yes, from the ICLR guidelines, they prefer bold writing. all the mathematical preferences are in math_commands.tex}

\begin{equation*}
% \label{eq:apx_bayes}
\begin{aligned}
p(\vtheta \mid \gD) &= \frac{p(\vtheta_1, \vtheta_2, \vtheta_s, \gD)}{p(\gD)}  \\
&\propto p(\vtheta_1 \mid \vtheta_2, \vtheta_s, \gD) p(\vtheta_2, \vtheta_s, \gD) \\
&= {p(\vtheta_1 \mid  \vtheta_s, \gD) p(\gD \mid \vtheta_2, \vtheta_s) p(\vtheta_2, \vtheta_s)} \\
&\propto \frac{p(\vtheta_1, \vtheta_s, \gD) p(\gD \mid \vtheta_2, \vtheta_s) p(\vtheta_2, \vtheta_s)}{p(\gD, \vtheta_s)} \\
&\propto \frac{p(\vtheta_1, \vtheta_s, \gD) p(\gD \mid \vtheta_2, \vtheta_s) p(\vtheta_2, \vtheta_s)}{\int p(\gD \mid \vtheta_1, \vtheta_s) p(\vtheta_s, \vtheta_1) d\vtheta_1} \\
&\propto \frac{p(\vtheta_1, \vtheta_s \mid \gD) p(\gD \mid \vtheta_2, \vtheta_s) p(\vtheta_2, \vtheta_s)}{\int p(\gD \mid \vtheta_1, \vtheta_s) p(\vtheta_s, \vtheta_1) d\vtheta_1},
\end{aligned}
\end{equation*}
where we used the conditional independence assumption  $p(\vtheta_1 \mid \vtheta_2, \vtheta_s, \gD) = p(\vtheta_1 \mid \vtheta_s, \gD)$ in the third line.
\end{proof}
%Using Bayes' theorem, we have
%\begin{equation*}
%% \label{eq:apx_bayes}
%\begin{aligned}
%p(\theta \mid \gD) &= \frac{p(\theta_1, \theta_2, \theta_s, %\gD)}{p(\gD)}  \\
%&= \frac{p(\theta_1 \mid \theta_2, \theta_s, \gD) p(\theta_2, \theta_s, %\gD)}{p(\gD)} \\
%&= \frac{p(\theta_1 \mid  \theta_s, \gD) p(\gD \mid \theta_2, \theta_s) %p(\theta_2, \theta_s)}{p(\gD)} \\
%&\propto \frac{p(\theta_1, \theta_s, \gD) p(\gD \mid \theta_2, %\theta_s) p(\theta_2, \theta_s)}{p(\gD, \theta_s)} \\
%&\propto \frac{p(\theta_1, \theta_s, \gD) p(\gD \mid \theta_2, %\theta_s) p(\theta_2, \theta_s)}{\int p(\gD \mid \theta_1, \theta_s) %p(\theta_s, \theta_1) d\theta_1} \\
%&\propto \frac{p(\theta_1, \theta_s \mid \gD) p(\gD \mid \theta_2, %\theta_s) p(\theta_2, \theta_s)}{\int p(\gD \mid \theta_1, \theta_s) %p(\theta_s, \theta_1) d\theta_1},
%\end{aligned}
%\end{equation*}
%where we used the conditional independence assumption in the third equality: $p(\theta_1 \mid \theta_2, \theta_s, \gD) = p(\theta_1 \mid \theta_s, \gD)$.
%\end{proof}

We now derive a closed-form expression for the denominator  of \eqref{eq:bayes2}.

% \begin{lemma}
%  Let us assume that we can obtain the maximum likelihood estimate $(\hat{\theta}_1, \hat{\theta}_s)$ for the first model. Then, let $Card(\theta_1) + Card(\theta_s) = p_1 + p_s = p$, and let the negative Hessian $H_p(\hat{\theta}_1, \hat{\theta}_s)$ of the $\log$ posterior probability distribution $\log p(\theta_1, \theta_s \mid \gD)$ evaluated at this maximum likelihood estimate be partitioned into four blocks corresponding to $(\theta_1, \theta_s)$ as
% \[
% H_p(\hat{\theta}_1, \hat{\theta}_s)=
% \left[
% \begin{array}{c|c}
% H_{11} & H_{1s} \\
% \hline
% H_{s1} & H_{ss}
% \end{array}
% \right].
% \]
% Under the assumptions that the weights of each model follow a Normal distribution, i.e., $(\theta_1, \theta_s) \sim \mathcal{N}_p(0, \sigma^2 I_p)$, with $I_p$ the $p$-dimensional identity matrix, 
 
% we have that
% \begin{equation*}
% \int p(\gD \mid \theta_1, \theta_s) p(\theta_s, \theta_1) d\theta_1 = e^{l_p(\hat{\theta}_1, \hat{\theta}_s) -\frac{1}{2}v^T\Omega v}  \times (2\pi)^{p_1/2} \lvert \det(H_{11}^{-1})\rvert^{1/2},
% \end{equation*}
% where $v = \theta_s - \hat{\theta}_s$ and $\Omega = H_{ss} - H_{1s}^TH_{11}^{-1} H_{1s}$.
% \end{lemma}

\begin{restatable}{lemma}{lemmatwo}
	\label{lem2} Suppose we have the maximum likelihood estimate $(\hat{\vtheta}_1, \hat{\vtheta}_s)$ for the first model, write $\mathrm{Card}(\vtheta_1) + \mathrm{Card}(\vtheta_s) = p_1 + p_s = p$, and let the negative Hessian $\mH_p(\hat{\vtheta}_1, \hat{\vtheta}_s)$ of the log posterior probability distribution $\log p(\vtheta_1, \vtheta_s \mid \mathcal{D})$ evaluated at $(\hat{\vtheta}_1, \hat{\vtheta}_s)$ be partitioned into four blocks corresponding to $(\vtheta_1, \vtheta_s)$ as\vspace{-1mm}
	\[
	\mH_p(\hat{\vtheta}_1, \hat{\vtheta}_s)=
	\left[
	\begin{array}{c|c}
	\mH_{11} & \mH_{1s} \\
	\hline
	\mH_{s1} & \mH_{ss}
	\end{array}
	\right].
	\]
	If the parameters of each model follow Normal distributions, i.e., $(\vtheta_1, \vtheta_s) \sim \mathcal{N}_p(\mathbf{0}, \sigma^2 \mI_p)$, with $\mI_p$ the $p$-dimensional identity matrix, 
	then \ky{the denominator of~\eqref{eq:bayes2}, $A = \int p(\mathcal{D} \mid \vtheta_1, \vtheta_s) p(\vtheta_s, \vtheta_1) d\vtheta_1$ can be written as}
	\begin{equation}
	A = \exp{\{  l_p(\hat{\vtheta}_1, \hat{\vtheta}_s) -\frac{1}{2}\vv^\top\mOmega \vv\}}  \times (2\pi)^{p_1/2} \lvert \det(\mH_{11}^{-1})\rvert^{1/2},
	\end{equation}
	where $\vv = \vtheta_s - \hat{\vtheta}_s$ and $\mOmega = \mH_{ss} - \mH_{1s}^\top\mH_{11}^{-1} \mH_{1s}$\ .
\end{restatable}

\begin{proof}
We have
\begin{equation*}
	\begin{aligned}
		p(\gD \mid \vtheta_1, \vtheta_s) p(\vtheta_s, \vtheta_1) &\propto e^{l(\vtheta_1, \vtheta_s) - (\vtheta_1, \vtheta_s)^T(\vtheta_1, \vtheta_s)/2\sigma^2} \\
		&\propto  e^{l_p(\vtheta_1, \vtheta_s)},
	\end{aligned}
\end{equation*}
where $l(\vtheta_1, \vtheta_s) = \log p(\gD \mid \vtheta_1, \vtheta_s)$, and $l_p(\vtheta_1, \vtheta_s) = l(\vtheta_1, \vtheta_s) - (\vtheta_1, \vtheta_s)^T(\vtheta_1, \vtheta_s)/2\sigma^2$. 

Let $\mH_p(\vtheta_1, \vtheta_s) = \mH(\vtheta_1, \vtheta_s) + \sigma^{-2}\mI_p$ be the negative Hessian of $l_p(\vtheta_1, \vtheta_s)$, with $\mI_p$ the $p$-dimensional identity matrix and $\mH(\vtheta_1, \vtheta_s)$ the negative Hessian of $l(\vtheta_1, \vtheta_s)$.

%\MS{What is $\mH$?}
Using the second-order Taylor expansion of $l_p(\vtheta_1, \vtheta_s)$ around its maximum likelihood estimate $(\hat{\vtheta}_1, \hat{\vtheta}_s)$, we have
\begin{equation}
% \label{eq:apx_taylor}
\begin{aligned}
l_p(\vtheta_1, \vtheta_s) &= l_p(\hat{\vtheta}_1, \hat{\vtheta}_s) -\frac{1}{2} (\vtheta_1', \vtheta_s')^T \mH_p(\hat{\vtheta}_1, \hat{\vtheta}_s)(\vtheta_1', \vtheta_s');
\end{aligned}
\end{equation}
where $(\vtheta_1', \vtheta_s') = (\vtheta_1, \vtheta_s) - (\hat{\vtheta}_1, \hat{\vtheta}_s)$.
The first derivative is zero since it is evaluated at the maximum likelihood estimate.
We now partition our negative Hessian matrix as 
\[
\mH_p(\hat{\vtheta}_1, \hat{\vtheta}_s)=
\left[
\begin{array}{c|c}
\mH_{11} & \mH_{1s} \\
\hline
\mH_{s1} & \mH_{ss}
\end{array}
\right],
\]
which gives
\begin{equation*}
\begin{aligned}
\mB =& [(\vtheta_1, \vtheta_s) - (\hat{\vtheta}_1, \hat{\vtheta}_s)]^T \mH_p(\hat{\vtheta}_1, \hat{\vtheta}_s)[(\vtheta_1, \vtheta_s) - (\hat{\vtheta}_1, \hat{\vtheta}_s)] \\
=&  (\vtheta_1 - \hat{\vtheta}_1)^T\mH_{11}(\vtheta_1 - \hat{\vtheta}_1) + (\vtheta_s - \hat{\vtheta}_s)^T\mH_{ss}(\vtheta_s - \hat{\vtheta}_s) \\ 
&\quad + (\vtheta_s - \hat{\vtheta}_s)^T\mH_{s1}(\vtheta_1 - \hat{\vtheta}_1) 
\\ &\quad +(\vtheta_1 - \hat{\vtheta}_1)^T\mH_{1s}(\vtheta_s - \hat{\vtheta}_s) \\
=&  (\vtheta_1 - \hat{\vtheta}_1)^T\mH_{11}(\vtheta_1 - \hat{\vtheta}_1) + (\vtheta_s - \hat{\vtheta}_s)^T\mH_{ss}(\vtheta_s - \hat{\vtheta}_s) \\ 
&\quad + (\vtheta_1 - \hat{\vtheta}_1)^T(\mH_{1s} + \mH_{s1}^T)(\vtheta_s - \hat{\vtheta}_s).
\end{aligned}
\end{equation*}
Let us define $\vu= \vtheta_1 - \hat{\vtheta}_1$, $\vv = \vtheta_s - \hat{\vtheta}_s$
and $\vw = \mH_{11}^{-1}\mH_{1s}\vv$. We then have,
\begin{equation*}
\begin{aligned}
\mC =&  (\vu+\vw)^T\mH_{11}(\vu+\vw)\\
=& \vu^T\mH_{11}\vu + \vu^T\mH_{11}\vw + \vw^T\mH_{11}\vw + \vw^T\mH_{11}\vu \\
=& (\vtheta_1 - \hat{\vtheta}_1)^T \mH_{11}(\vtheta_1 - \hat{\vtheta}_1)  \\ 
&\quad + (\vtheta_1 - \hat{\vtheta}_1)^T \mH_{11}\mH_{11}^{-1}\mH_{1s}(\vtheta_s - \hat{\vtheta}_s)  \\ 
&\quad + \vv^T\mH_{1s}^T\mH_{11}^{-1}\mH_{11}\mH_{1s}\vv \\ 
&\quad + \vv^T\mH_{1s}^T\mH_{11}^{-1}\mH_{11}(\vtheta_1 - \hat{\vtheta}_1) \\
=&  \mB - \vv^T\mH_{ss}\vv + \vv^T\mH_{1s}^TH_{11}^{-1}\mH_{1s}\vv \\
=& \mB -\vv^T(\mH_{ss} - \mH_{1s}^T\mH_{11}^{-1} \mH_{1s})v \\
=& \mB -\vv^T\mOmega \vv,
\end{aligned}
\end{equation*}
with $\mOmega = \mH_{ss} - \mH_{1s}^T\mH_{11}^{-1} \mH_{1s}$.

Thus
\begin{equation}
 \label{eq:apx_a}
\mB=(\vu+\mH_{11}^{-1}\mH_{1s}v)^T\mH_{11}(\vu+\mH_{11}^{-1}\mH_{1s}\vv) + \vv^T\mOmega \vv.
\end{equation}

Given \eqref{eq:apx_a}, we are now able to prove Lemma \ref{lem2}, as integral 
\begin{equation*}
\begin{aligned}
D &= \int e^{l_p(\vtheta_1, \vtheta_s)} d\vtheta_1 =  \int e^{l_p(\hat{\vtheta}_1, \hat{\vtheta}_s) - \frac{1}{2}\mB} d\vtheta_1   \\
&= \int e^{l_p(\hat{\vtheta}_1, \hat{\vtheta}_s)} e^{-\frac{1}{2}\mB } d\vtheta_1 =  e^{l_p(\hat{\vtheta}_1, \hat{\vtheta}_s)}\int e^{-\frac{1}{2}\mB} d\vtheta_1 \\
&=  \int e^{-\frac{1}{2}((\vu+\mH_{11}^{-1}\mH_{1s}\vv)^T\mH_{11}(\vu+\mH_{11}^{-1}\mH_{1s}\vv) + \vv^T\mOmega \vv)} d\vtheta_1  \\
& \quad \quad \times e^{l_p(\hat{\vtheta}_1, \hat{\vtheta}_s)} \\
&= \int e^{-\frac{1}{2}((\vu+\mH_{11}^{-1}\mH_{1s}\vv)^T\mH_{11}(\vu+\mH_{11}^{-1}\mH_{1s}\vv))}e^{-\frac{1}{2}\vv^T\mOmega \vv} d\vtheta_1 \\
& \quad \quad \times e^{l_p(\hat{\vtheta}_1, \hat{\vtheta}_s)} \\
&= e^{l_p(\hat{\vtheta}_1, \hat{\vtheta}_s) -\frac{1}{2}\vv^T\mOmega \vv} \int e^{-\frac{1}{2}(\vtheta_1 - \vz)^T\mH_{11}(\vtheta_1 - \vz)}d\vtheta_1 \\
 &=  e^{l_p(\hat{\vtheta}_1, \hat{\vtheta}_s) -\frac{1}{2}\vv^T\mOmega \vv} (2\pi)^{\frac{p_1}{2}} \lvert \det(\mH_{11}^{-1})\rvert^{\frac{1}{2}} \\
 & \quad \quad \times (2\pi)^{-\frac{p_1}{2}} \lvert\det(\mH_{11}^{-1})\rvert^{-\frac{1}{2}} \\
 & \quad \quad \times  \int e^{-\frac{1}{2}(\vtheta_1 - \vz)^T\mH_{11}(\vtheta_1 - \vz)}d\vtheta_1   \\
&= e^{l_p(\hat{\vtheta}_1, \hat{\vtheta}_s) -\frac{1}{2}\vv^T\mOmega \vv} (2\pi)^{\frac{p_1}{2}} \lvert \det(\mH_{11}^{-1})\rvert^{\frac{1}{2}},
\end{aligned}
\end{equation*}
where we re-arranged the terms so that the integral is over a normal distribution with mean $\vz=\hat{\vtheta}_1 - \mH_{11}^{-1}\mH_{1s}(\vtheta_s - \hat{\vtheta}_s)$ and covariance matrix $\mH_{11}^{-1}$, which can be computed in closed form.
% \MS{Correct?} Yes 
%where we arranged the scaling in order to integrate over the normal distribution with mean $z$ and covariance matrix $H_{11}^{-1}$ with $z=\hat{\theta}_1 - H_{11}^{-1}H_{1s}(\theta_s - \hat{\theta}_s)$.
\end{proof}

From Lemma~\ref{lem1} and Lemma~\ref{lem2}, we can obtain equation 3 by replacing the denominator with the closed form above and taking the $\log$ on both size of \eqref{eq:bayes2}. This yields
\begin{align*}
    \log p(\vtheta | \gD) &\propto \log{p(\gD \mid \vtheta_2, \vtheta_s)} + \log{p(\vtheta_1, \vtheta_s)} \\ 
    & \quad \quad + \log{p(\vtheta_2, \vtheta_s)} \\ 
    & \quad \quad - \log{\{\int p(\gD \mid \vtheta_1, \vtheta_s) p(\vtheta_1, \vtheta_s) d\vtheta_1 \}} \\
    &= \log{p(\gD \mid \vtheta_2, \vtheta_s)} + \log{p(\vtheta_1, \vtheta_s)}  \\ 	
	&    \quad \quad + \log{p(\vtheta_2, \vtheta_s)}  - l_p(\hat{\vtheta}_1, \hat{\vtheta}_s) + \frac{1}{2}\vv^T\mOmega \vv \\
    &\propto \log p(\gD \mid \vtheta_2, \vtheta_s)  + \log p(\vtheta_2, \vtheta_s) \\ 
    & \quad \quad +\log p(\vtheta_1, \vtheta_s \mid \gD)  +  \frac{1}{2}\vv^T \mOmega \vv\;.
\end{align*}

\begin{figure*}
    \centering
    \includegraphics[width=\textwidth]{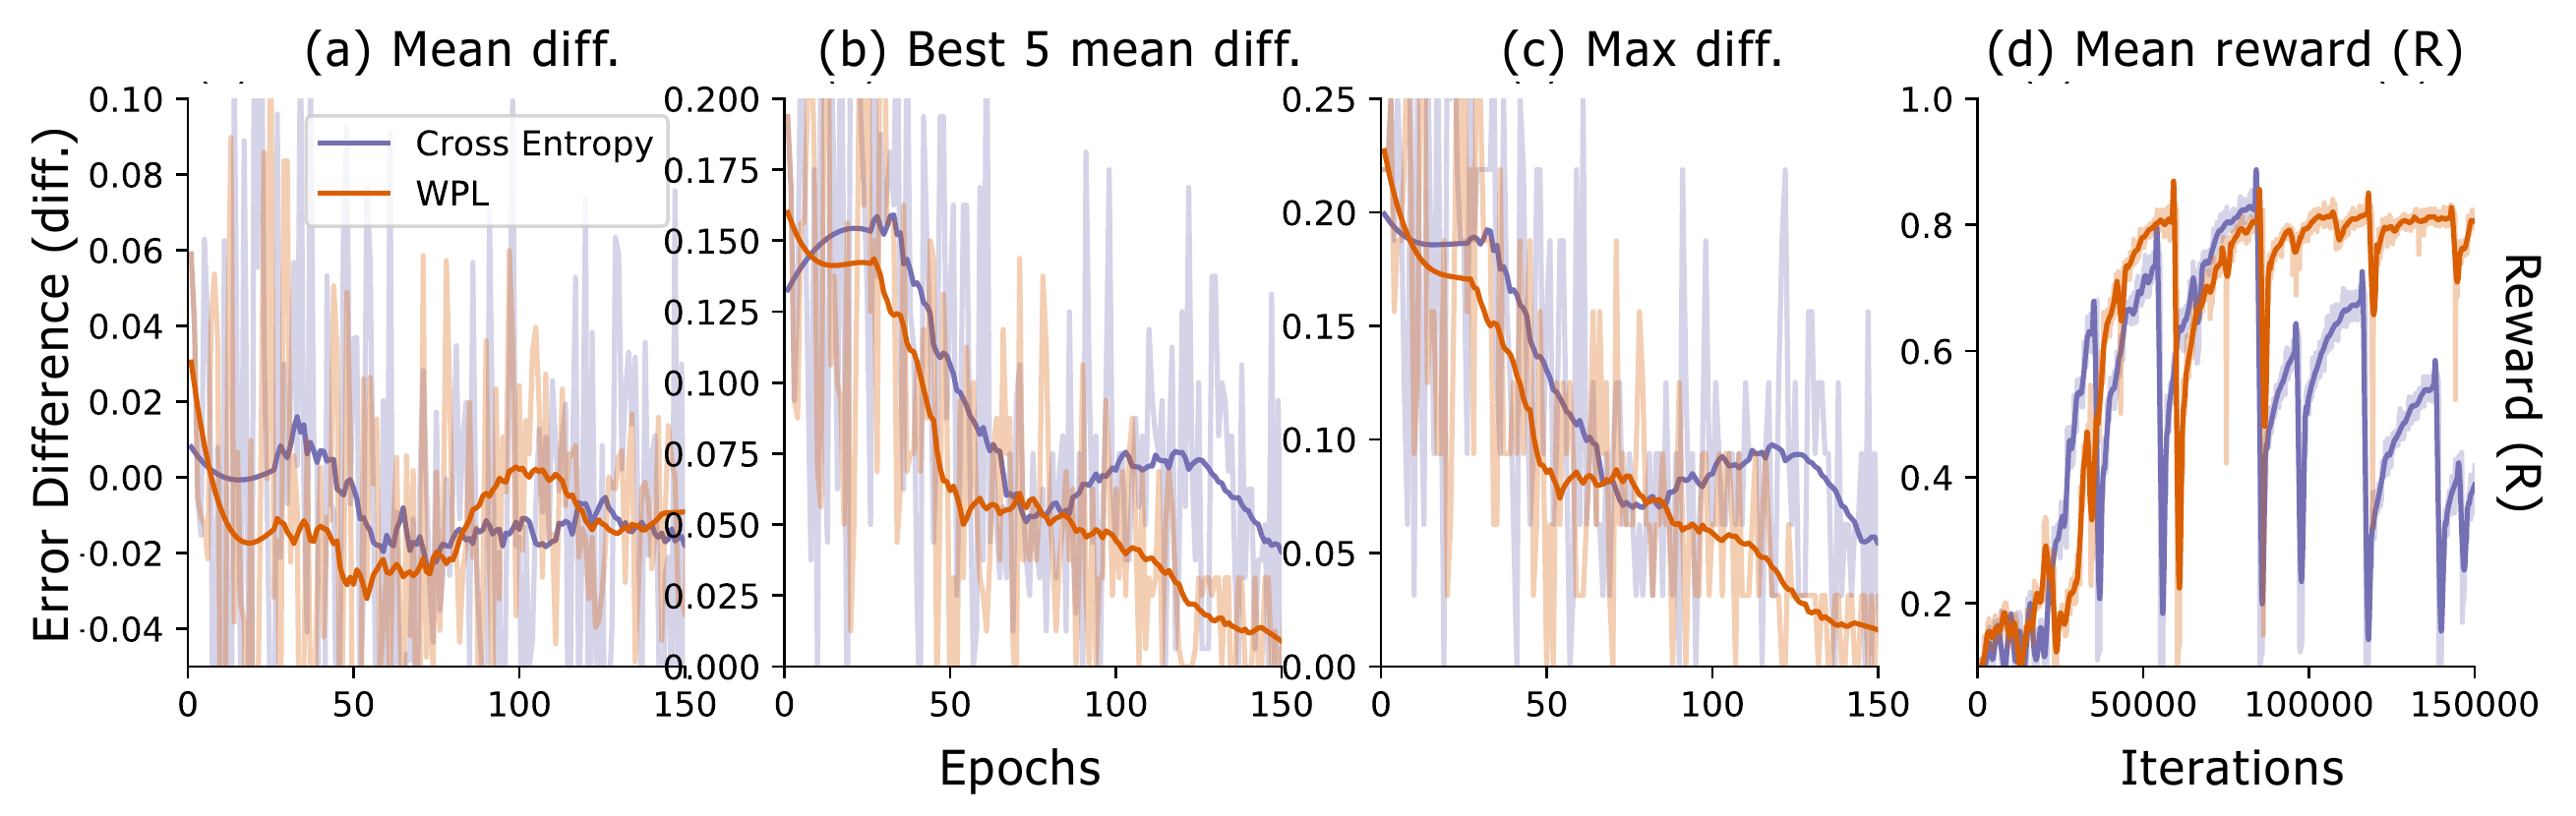}
    \caption{\textbf{Error differences when searching for CNN architectures.}
    Quantitatively, the multi-model forgetting effect is reduced by up to 99\% for \captiona, 96\% for \captionb, and 98\% for \captionc.}
    \label{fig:cnn_final}
\end{figure*}

\section{Plots for CNN Search}
In our CNN search experiment, we search for a``micro" cell as in \citep{Pham18}. We employ the hyper-parameters available in the released ENAS code. The plots depicting error difference as a function of training epochs as provided in~\Figref{fig:cnn_final}~\captiona,~\captionb and~\captionc. Note that here again the original ENAS is subject to multi-model forgetting, and our WPL helps reducing it. In~\Figref{fig:cnn_final}~\captiond, we show the mean reward as training progresses. While the shape of the reward curve is different from the RNN case, because of a different formulation of the reward function, the general trend is the same; Our approach initially produces lower rewards, but is better at maintaining good models until the end of the search, as indicated by higher rewards in the second half of training.
%Due to the formulation of rewards is different, training behavior differs from the RNN cell, but our conclusion remains the same as RNN case. With the help of WPL, the brainwashing effect is reduced to a minimal level as in~\Figref{fig:cnn_final}~\captiona,~\captionb and~\captionc, and furthermore, it helps the model converge in more stable way, as shown in~\Figref{fig:cnn_final}~\captiond. 

\section{Best architectures found by the search}
In~\Figref{fig:best-arch}, we show the best architectures found by our neural architecture search for the RNN and CNN cases.
\begin{figure*}
    \centering
    \includegraphics[width=150mm]{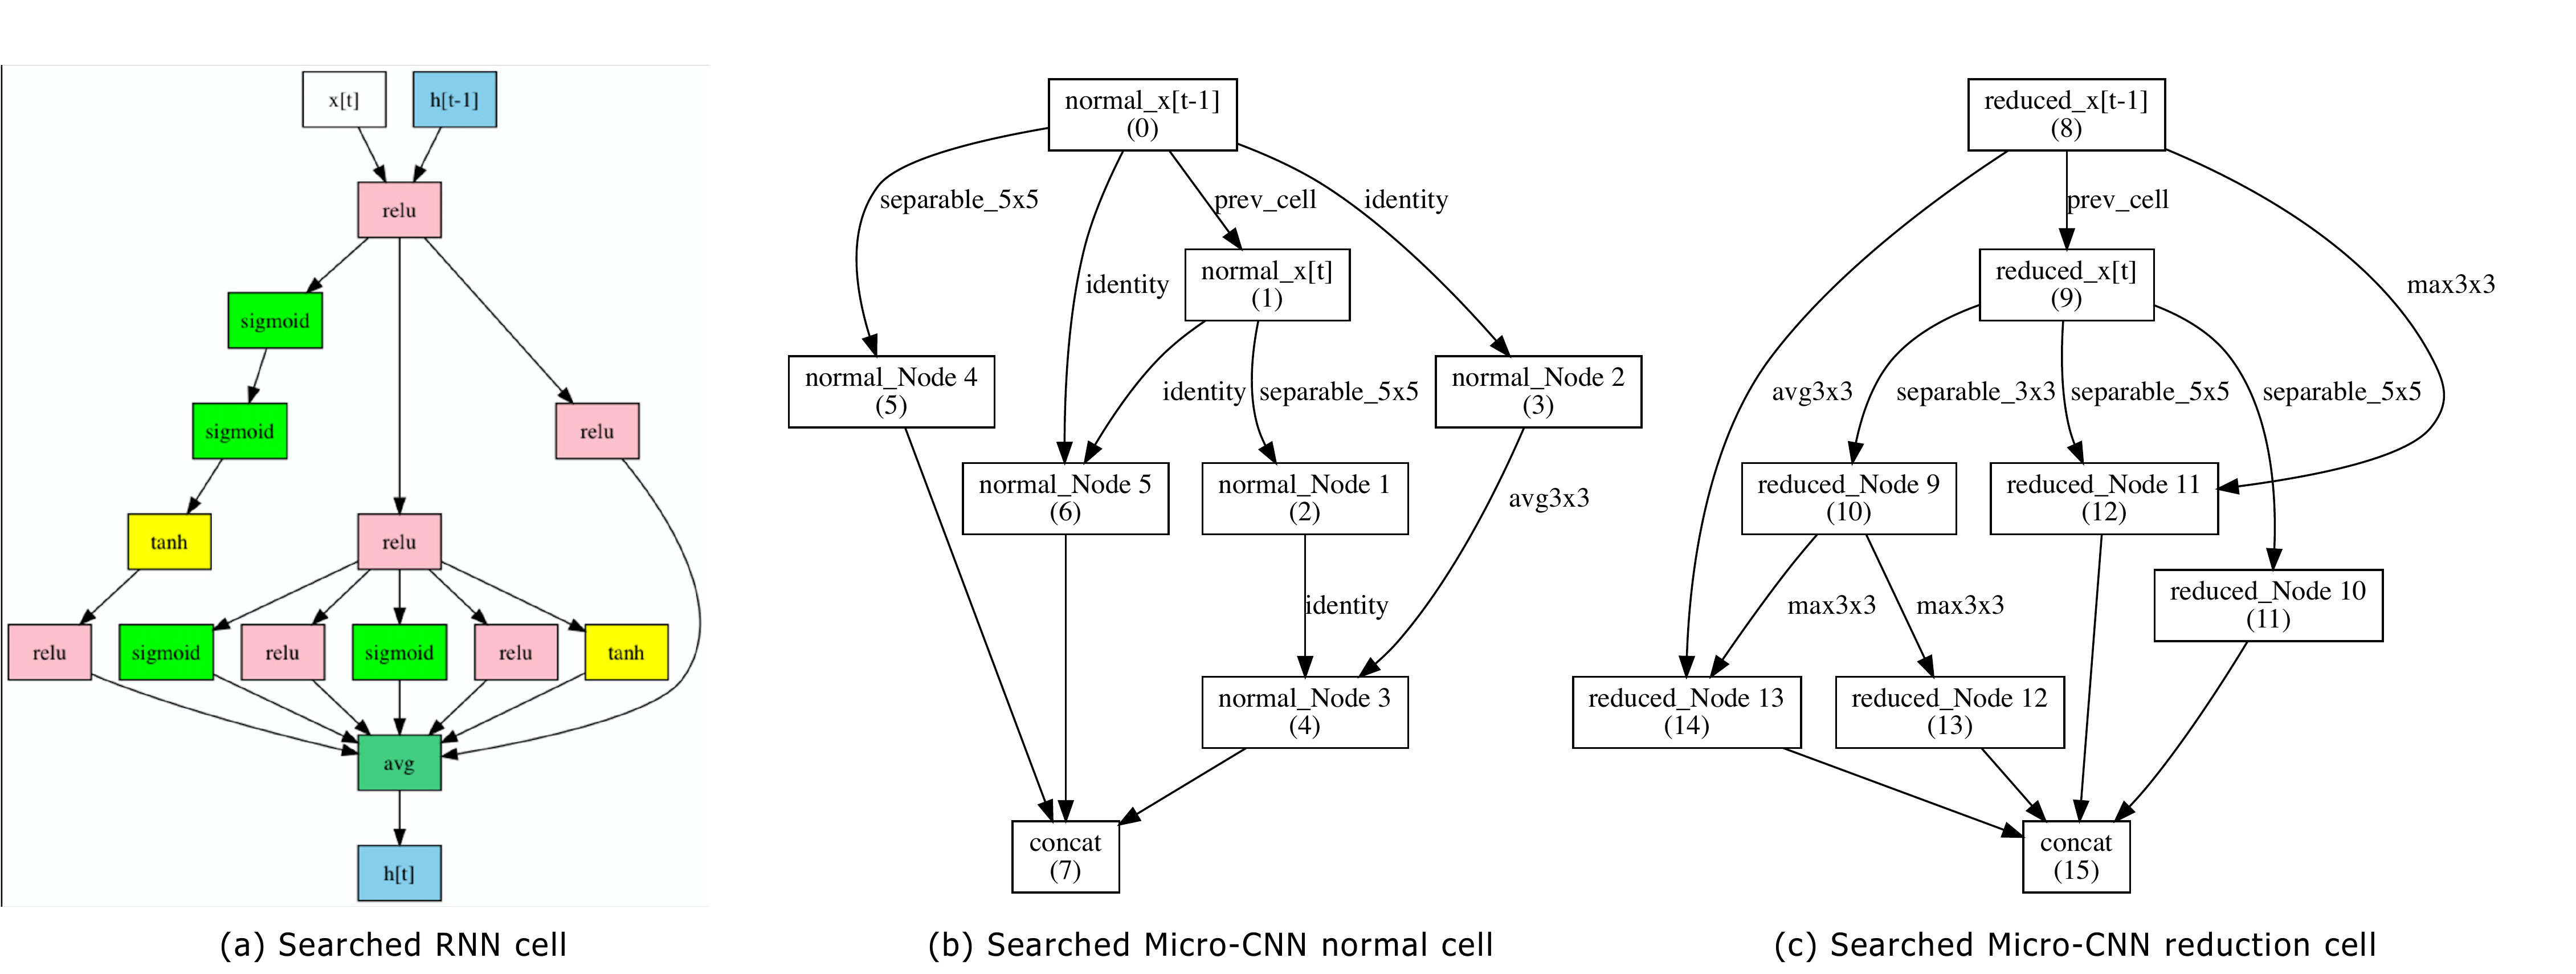}
    \caption{\textbf{Best architectures found for RNN and CNN.}
    We display the best architecture found by ENAS+WPL, in \captiona\ for the RNN cell, and in \captionb~and \captionc~for the CNN normal and reduction cells.
    }
    \label{fig:best-arch}
\end{figure*}

% \begin{figure}
%     \centering
%     \includegraphics[width=\textwidth]{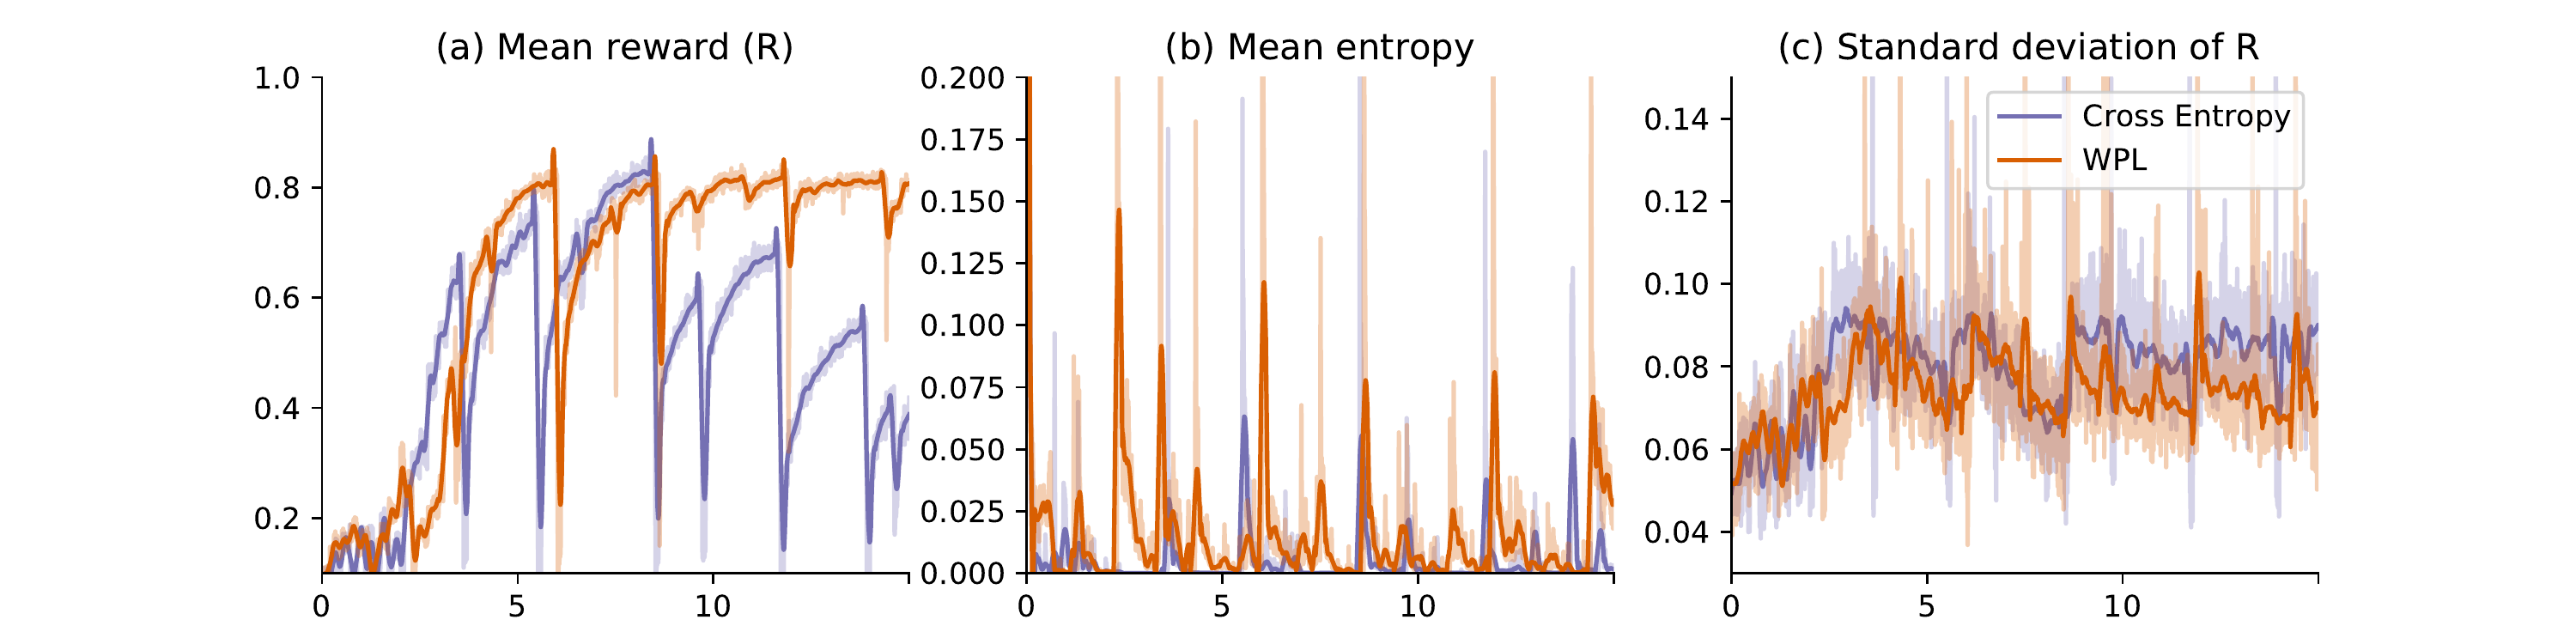}
%     \caption{\textbf{Visualizing the training of reinforcement learning controller of CNN.}}
%     \label{fig:my_label}
% \end{figure}
